# Supplementary material for: Parameter-free Mirror Descent
Source: arXiv:2203.00444 source file (2024-02-08)
Supplement: Supplementary file 1 [file appendix.tex]

%auto-ignore
\documentclass[paper]{subfiles}
\begin{document}

\appendix

\newtheorem{applemma}{Lemma}

\subfile{Appendices/strong-md-Dhat.tex}

\subfile{Appendices/centered-md.tex}
\subfile{Appendices/optimal-pf.tex}
\subfile{Appendices/dynamic.tex}
\subfile{Appendices/implicit.tex}
\subfile{Appendices/improved-scale-free.tex}
\subfile{Appendices/optimal-tradeoff.tex}
\subfile{Appendices/lemmas.tex}
\subfile{Appendices/dynamic-reduction.tex}
\subfile{Appendices/amortized-time.tex}

\end{document}
